# Supplementary material for: Carrier-number fluctuations in the 2-dimensional electron gas at the LaAlO3/SrTiO3 interface
Source: arXiv:1312.2181 source file (2013-12-08)
Supplement: Supplementary file 1 [file SupplementalMaterial.pdf]

# Carrier-number fluctuations in the 2-dimensional electron gas at the $LaAlO_3/SrTiO_3$ interface
# SUPPLEMENTAL MATERIAL

C. Barone[1], F. Romeo[1], S. Pagano[1], E. Di Gennaro[2], F. Miletto Granozio[2], I. Pallecchi[3], D. Marrè[3], and U. Scotti di Uccio[2]

*[1] Dipartimento di Fisica "E.R. Caianiello" and CNR-SPIN Salerno, Università di Salerno, I-84084 Fisciano, Salerno, Italy*
*[2] CNR-SPIN Napoli and Dipartimento di Scienze Fisiche, Università di Napoli "Federico II", I-80125 Napoli, Italy*
*[3] CNR-SPIN Genova and Dipartimento di Fisica, Università di Genova, I-16152 Genova, Italy*

**General properties of the noise spectral density**

Given a stochastic real signal x(t), such that $\langle x(t)\rangle = 0$ and $\langle x^2(t)\rangle = \sigma^2$, we define the noise spectral density, in terms of the Fourier transform $\tilde{x}(\omega)$, as $S_x(\omega) = \left\langle |\tilde{x}(\omega)|^2 \right\rangle$. This function satisfies the general normalization condition:

$$\int_0^\infty S_x(\omega)\, d\omega = \pi\, \sigma^2 \qquad (1)$$

**Explanation of the 1/f behavior of $S_N(\omega)$ for the 2DEG at LAO/STO interface**

We start from the assumption that the noise in 2DEGs at LAO/STO interface is basically due to carrier-number fluctuations. In order to determine $S_N(\omega)$, we consider the stochastic variable ΔN(t), representing the deviation of the number of the mobile electrons from its equilibrium value. The evolution in time of ΔN is described by a rate equation:

$$\frac{d}{dt}\Delta N = -\frac{\Delta N}{\tau} + \xi(t) \qquad (2)$$

Here, $\tau$ is a characteristic time for the equilibration of mobile electrons and traps. The function $\xi(t)$ describes the process of adding or subtracting one electron at subsequent times $t_i$, i.e., $\xi(t) = \sum_i \psi_i\, \delta(t - t_i)$ with $\psi_i = \pm 1$ and $\langle \psi_i \rangle = 0$ ; $\langle \psi_i\, \psi_j \rangle = \delta_{ij}$.

$\xi(t)$ is characterized by the ensemble averages $\left\langle \frac{1}{T}\int_{-T/2}^{T/2} \xi(t)\, dt \right\rangle = 0$ and $\left\langle \frac{1}{T}\int_{-T/2}^{T/2} \xi(t)\,\xi(t+t')\, dt \right\rangle = 2R\,\delta(t')$, where the constant R represent the average number of mobile electrons that are trapped per unit time.

By applying the Fourier transformation, the solution of the rate equation is readily found:

$$\Delta\tilde{N}(\omega) = \frac{\tilde{\xi}(\omega)\,\tau}{1 + i\,\omega\tau} \qquad (3)$$

Hence:

$$S_N(\omega) = \left\langle |\Delta\tilde{N}(\omega)|^2 \right\rangle = \frac{\left\langle |\tilde{\xi}(\omega)|^2 \right\rangle \tau^2}{1 + \omega^2\tau^2} = \frac{2R\,\tau^2}{1 + \omega^2\tau^2} \qquad (4)$$

Finally, due to the normalization rule of $S_N(\omega)$, we can get rid of R, and obtain:

$$S_N(\omega) = \frac{2\sigma^2\,\tau}{1 + \omega^2\tau^2} = \frac{2\,\sigma^2\,\tau}{1 + (2\pi\,\tau)^2 f^2} \qquad (5)$$

The expected spectrum will be the sum over the range of possible values for $\tau$. To determine this, we then consider the mechanism of excitation-trapping in oxides. We assume that the excitation from a trap is due to scattering with acoustic phonons, that carry negligible moment, i.e., it is vertical in the k-space. According to the sketch in Fig. 4 of the main text, that we copy here for convenience as Fig. (1), such process requires an activation energy $E_o$, that we assume as uniformly distributed above the threshold $E_a$. Therefore, we substitute $\tau = \tau_0 \exp\left(\frac{E_o}{k_B T}\right)$ in the previous formula of Eq. (5), and sum over the possible values of $E_o$. The energy scale is set by the average acoustic phonon energy $k_B T$. We then define $x = \frac{E_o}{k_B T}$, and integrate over dx. In view of the exponential dependence of $\tau$ on $E_o$, the lower integration limit can be approximated to 0 (the condition $\omega \tau_0 \exp\left(\frac{E_o}{k_B T}\right) << 1$ is always satisfied):

$$S_N(\omega) = \int_0^\infty dx \frac{2\sigma^2 \tau}{1+\omega^2\tau^2} = \int_{\tau_o}^\infty \frac{2\sigma^2 \, d\tau}{1+\omega^2\tau^2} \approx \frac{\pi \sigma^2}{\omega} = \frac{\sigma^2}{2f} \qquad (6)$$

This expression shows the 1/f dependence that is observed in experiments.

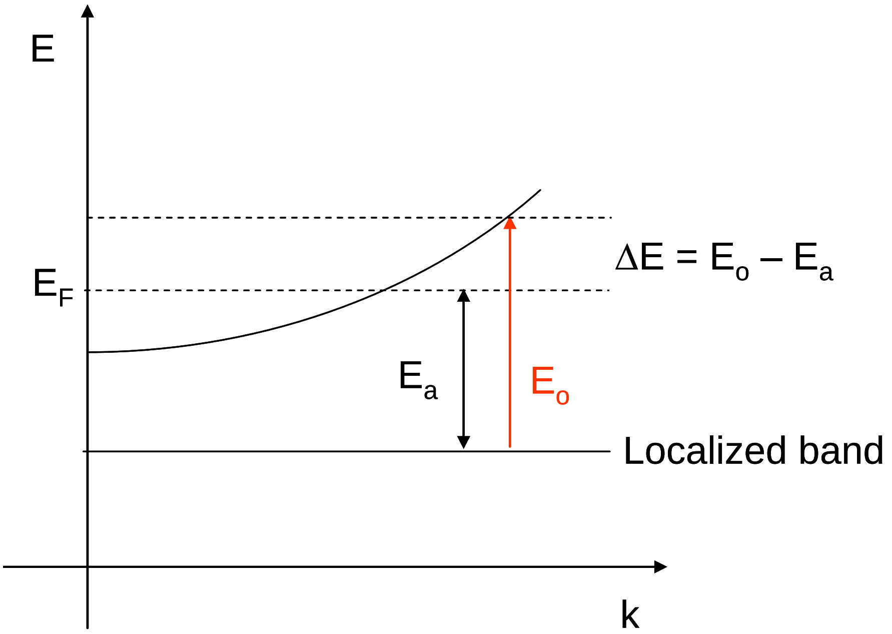


**Fig. (1):** Sketch of the activation process.

**The variance of mobile electrons number $\sigma^2$**

The simplest way to evaluate the variance of the mobile electrons number is to depict the system as a two-level statistical system: mobile states have energy $E_F$ and trap states lie at energy $E_F - E_a$. The partition function is $Z = \exp\left(-\frac{E_F}{k_B T}\right) + \exp\left(-\frac{E_F - E_a}{k_B T}\right)$. The probability to observe a single electron excited out of the trap is $p = Z^{-1} \exp\left(-\frac{E_F}{k_B T}\right)$, while the probability to observe a trapped electron is $q = Z^{-1} \exp\left(-\frac{E_F - E_a}{k_B T}\right)$.

Following Eq. (1) in the main text, we set $N_1 = A \cdot n_1$ as the number of trapped electrons, being A the effective sample area. The number of mobile electrons is given by a residual term $N_0 = A \cdot n_0$ added to the activated term $N_1 \exp\left(-\frac{E_a}{k_B T}\right)$.

In order to evaluate $\sigma^2$, i.e., the variance of the mobile carriers number, we first consider the expression of the binomial statistics for a population of $N_1$ particles that can jump from one state to the others (and the reverse) with probability p (and q). Then, we quadratically add the variance $\sigma_0^2$ of the residual term $N_0$. The result is:

$$\sigma^2 = \sigma^2_{N_1} + \sigma^2_{N_0} = N_1 p q + \sigma^2_0 \qquad (7)$$

When considering the explicit expression of p, q, and $N_1$, we note that the first term in this expression has a weak dependence on temperature and is considerably smaller than $\sigma_0^2$ . Fig. (2) shows a comparison of the noise experimental data with the fitting expression (see Eq. (3) in the main text) that assumes a constant $\sigma^2$ (red solid curve), and with the theoretical prediction using Eq. (7) of this Supplemental Materials (blue dashed curve). The closeness of the two curves is self evident.

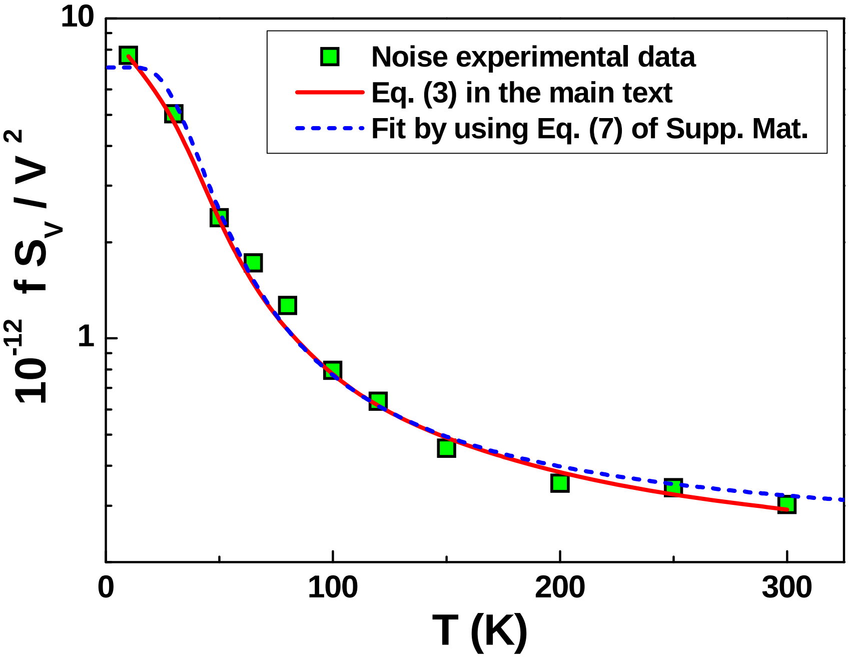


**Fig. (2):** Comparison between the noise experimental data, the fitting formula of Eq. (3) in the main text, and the fitting formula obtained by using Eq. (7) of this Supplemental Materials.
